# Supplementary material for: CROCODIL: Cross-Model Code Editing with LLMs
Source: arXiv:2609.03894 source file (2026-09-03)
Supplement: Supplementary file 2 [file edit_limit_guidelines.tex]

\begin{figure*}[t]
\noindent\rule{\linewidth}{\heavyrulewidth}
\vspace{-4pt}
\lstinputlisting[style=ContextSnippet]{figures/prompts/system_edit_limit_guidelines.md}
\vspace{-4pt}
\noindent\rule{\linewidth}{\heavyrulewidth}
\vspace{-8pt}
\caption{\UseMacro{FCap-prompt-edit-limit-guidelines}}
\label{fig:prompt-edit-limit-guidelines}
\end{figure*}
