# Supplementary material for: CROCODIL: Cross-Model Code Editing with LLMs
Source: arXiv:2609.03894 source file (2026-09-03)
Supplement: Supplementary file 3 [file instruct_plan_example.tex]

\begin{figure}[h]
\begin{subfigure}{\columnwidth}
\lstinputlisting[style=ContextSnippet,language=rust-pretty,numbersep=6pt]{figures/instruct_plan/fancy_regex_fmt_candidate.rs}
\caption{\UseMacro{FCap-instruct-plan-example-candidate}}
\label{fig:instruct-plan-example-candidate}
\end{subfigure}

\vspace{4pt}

\begin{subfigure}{\columnwidth}
\lstinputlisting[style=ContextSnippet]{figures/instruct_plan/fancy_regex_fmt_plan.txt}
\caption{\UseMacro{FCap-instruct-plan-example-plan}}
\label{fig:instruct-plan-example-plan}
\end{subfigure}
\vspace{-8pt}
\caption{\UseMacro{FCap-instruct-plan-example}}
\label{fig:instruct-plan-example}
\end{figure}
