# Supplementary material for: CROCODIL: Cross-Model Code Editing with LLMs
Source: arXiv:2609.03894 source file (2026-09-03)
Supplement: Supplementary file 4 [file qualitative.tex]

\begin{figure}[h]
        \begin{subfigure}{\columnwidth}
                \lstinputlisting[language=rust-diff]{figures/qualitative/scopedrift_endianness_base.rs}
                \caption{Base edit.}
                \label{fig:scopedrift-endianness-base}
        \end{subfigure}
        \begin{subfigure}{\columnwidth}
                \vspace{4mm}
                \lstinputlisting[language=rust-diff]{figures/qualitative/scopedrift_endianness_rl.rs}
                \caption{RL edit.}
                \label{fig:scopedrift-endianness-rl}
        \end{subfigure}
        \caption{Scope drift on \texttt{endianness} (\texttt{bytecode} \texttt{alliance}/\texttt{target}-\texttt{lexicon} PR \#79, \qwen \rewriter).  The \basemodel prefixes a fabricated enum definition with invalid pattern syntax; the \rlmodel writes only the one new match arm.}
        \label{fig:scopedrift-endianness}
        \vspace{6.5mm}
\end{figure}

\begin{figure}[h]
        \begin{subfigure}{\columnwidth}
                \lstinputlisting[language=rust-diff]{figures/qualitative/rename_cookedbytestring_base.rs}
                \caption{Base edit.}
                \label{fig:rename-cookedbytestring-base}
        \end{subfigure}
        \begin{subfigure}{\columnwidth}
                \vspace{4mm}
                \lstinputlisting[language=rust-diff]{figures/qualitative/rename_cookedbytestring_rl.rs}
                \caption{RL edit.}
                \label{fig:rename-cookedbytestring-rl}
        \end{subfigure}
        \caption{Partial rename on \texttt{cooked}\texttt{\_byte}\texttt{\_string} (\texttt{dtolnay}/\texttt{proc-macro2} PR \#282, \qwen \rewriter).  The PR renames \texttt{LexError} to \texttt{Reject}; the \rlmodel keeps the old return type and additionally introduces an unterminated character literal.}
        \label{fig:rename-cookedbytestring}
\end{figure}
